# Supplementary material for: Monadic Decomposition in Integer Linear Arithmetic (Technical Report)
Source: arXiv:2004.12371 source file (2020-04-26)
Supplement: Supplementary file 1 [file appendix.tex]

\input{inf-sols}
\input{variadic-completeness}
